# Supplementary material for: Depends-Kotlin: A Cross-Language Kotlin Dependency Extractor
Source: arXiv:2401.16865 source file (2024-08-21)
Supplement: Supplementary file 1 [file appendix.tex]

\appendix

\section{Walkthrough}

\subsection{Download and Build}
\textit{Depends-Kotlin} can be built and run by following 3 steps.
\begin{description}
    \item[Step 1.]  Clone repository
\end{description}
Our repository is hosted on GitHub, you can clone the source code with the following command:

\lstinline[language=bash]|git clone https://github.com/XYZboom/depends-kotlin.git|

\begin{description}
    \item[Step 2.] Compile project
\end{description}
Before compiling the project, make sure you have the Java 17 runtime ready. After that, run the following command at the root of your project to compile it:

on Windows
\begin{center}
    \lstinline[language=bash]|gradlew.bat build| \\
\end{center}

on Linux
\begin{center}
    \lstinline[language=bash]|gradlew build|
\end{center}

Meanwhile, the \verb|-x test| option can be used to skip testing. At this point, Gradle Wapper will pull the necessary dependencies and compile them. If everything goes smoothly, you will see an output like this.

\begin{figure}[H]
    \centering
    \includegraphics[width=\columnwidth]{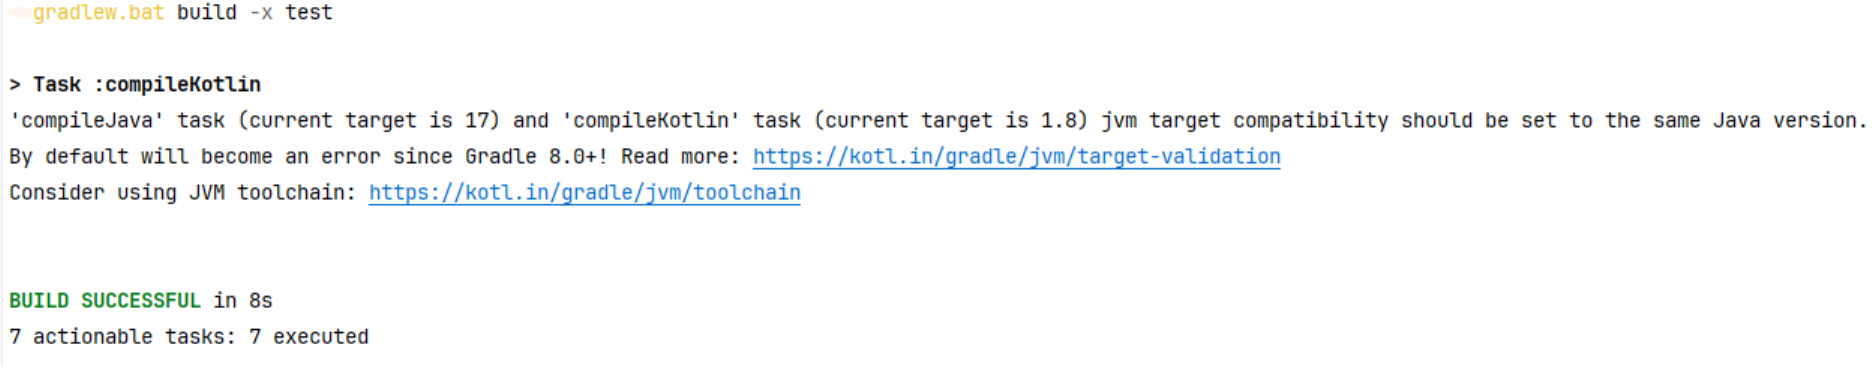}
    \caption{Screenshot of \textit{Depends-Kotlin}'s compilation.}
    \label{fig:compile}
\end{figure}

\begin{description}
    \item[Step 3.] Generate Runnable Jar
\end{description}
After successful compilation, you can use Gradle's shadow plugin to package it as an executable jar using the following command:

on Windows
\begin{center}
    \lstinline[language=bash]|gradlew.bat shadowJar| \\
\end{center}

on Linux
\begin{center}
    \lstinline[language=bash]|gradlew shadowJar|
\end{center}

You will see the following output and find an executable jar package with the suffix \texttt{*. all.jar} in the \verb|projectRoot/build/libs| folder.

\begin{figure}[H]
    \centering
    \includegraphics[width=\columnwidth]{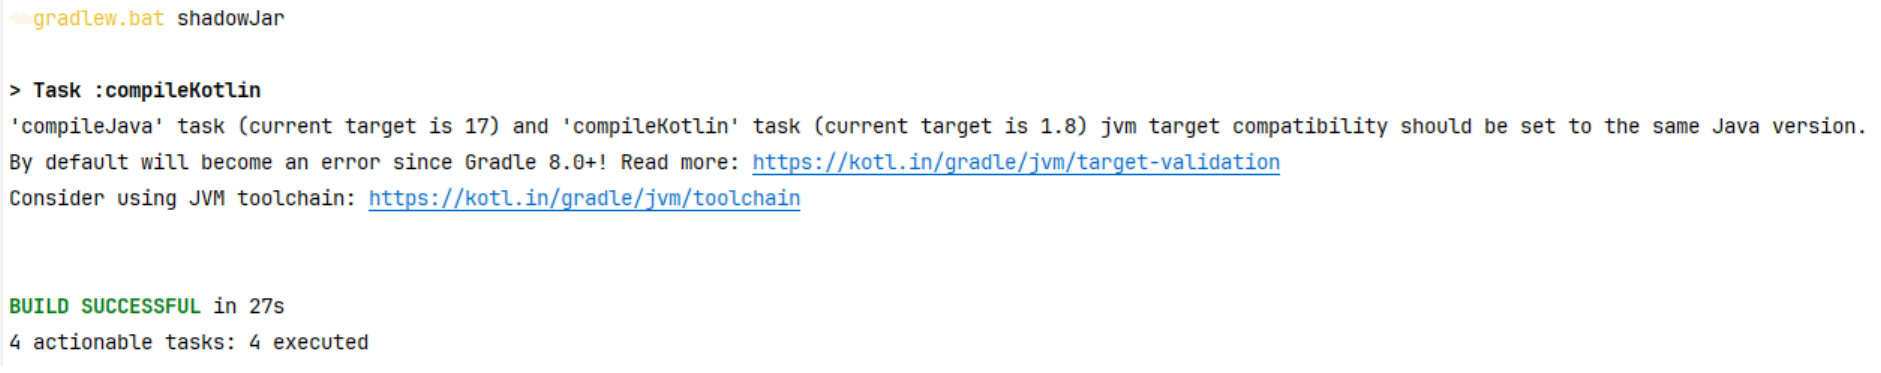}
    \caption{Screenshot of \textit{Depends-Kotlin}'s packaging.}
    \label{fig:shadow}
\end{figure}

\subsection{Run from Command Line}
\textit{Depends-Kotlin} is based on the JVM platform and requires at least Java 17. The input of \textit{Depends-Kotlin} is the source folder path of a particular project. The full command line arguments are as follows:
\begin{verbatim}
Usage: depends <lang> <src> <output> [OPTIONS] 
Options:
\end{verbatim}

\begin{tabular}{@{}ll}
    \texttt{--auto-include} &Auto include all paths under \\
    \texttt{} &the source path\\
    \texttt{-h, -{}--help} & Show this message and exit \\
    \texttt{-i, -{}--include} &  The files of searching path \\
    \texttt{-d, -{}--dir} &  The output directory \\
    \texttt{-f, -{}--format} & The output format\\
    \texttt{-g, -{}--granularity} &Granularity of dependency \\
    \texttt{-s, -{}--strip-leading-path} & Strip the leading path \\
    \texttt{-{}--show-language} & Show language info in dependency type \\
    \texttt{-m, -{}--n-map-files} & Output DV8 dependency map file \\
    \texttt{-p, -{}--namepattern} & The name path separators \\
\end{tabular}

\begin{verbatim}
Arguments:
 lang                 The language of project files
 src                  The directory to be analyzed
 output               The output file name
\end{verbatim}

\begin{figure}[t]
    \centering
    \includegraphics[width=\linewidth]{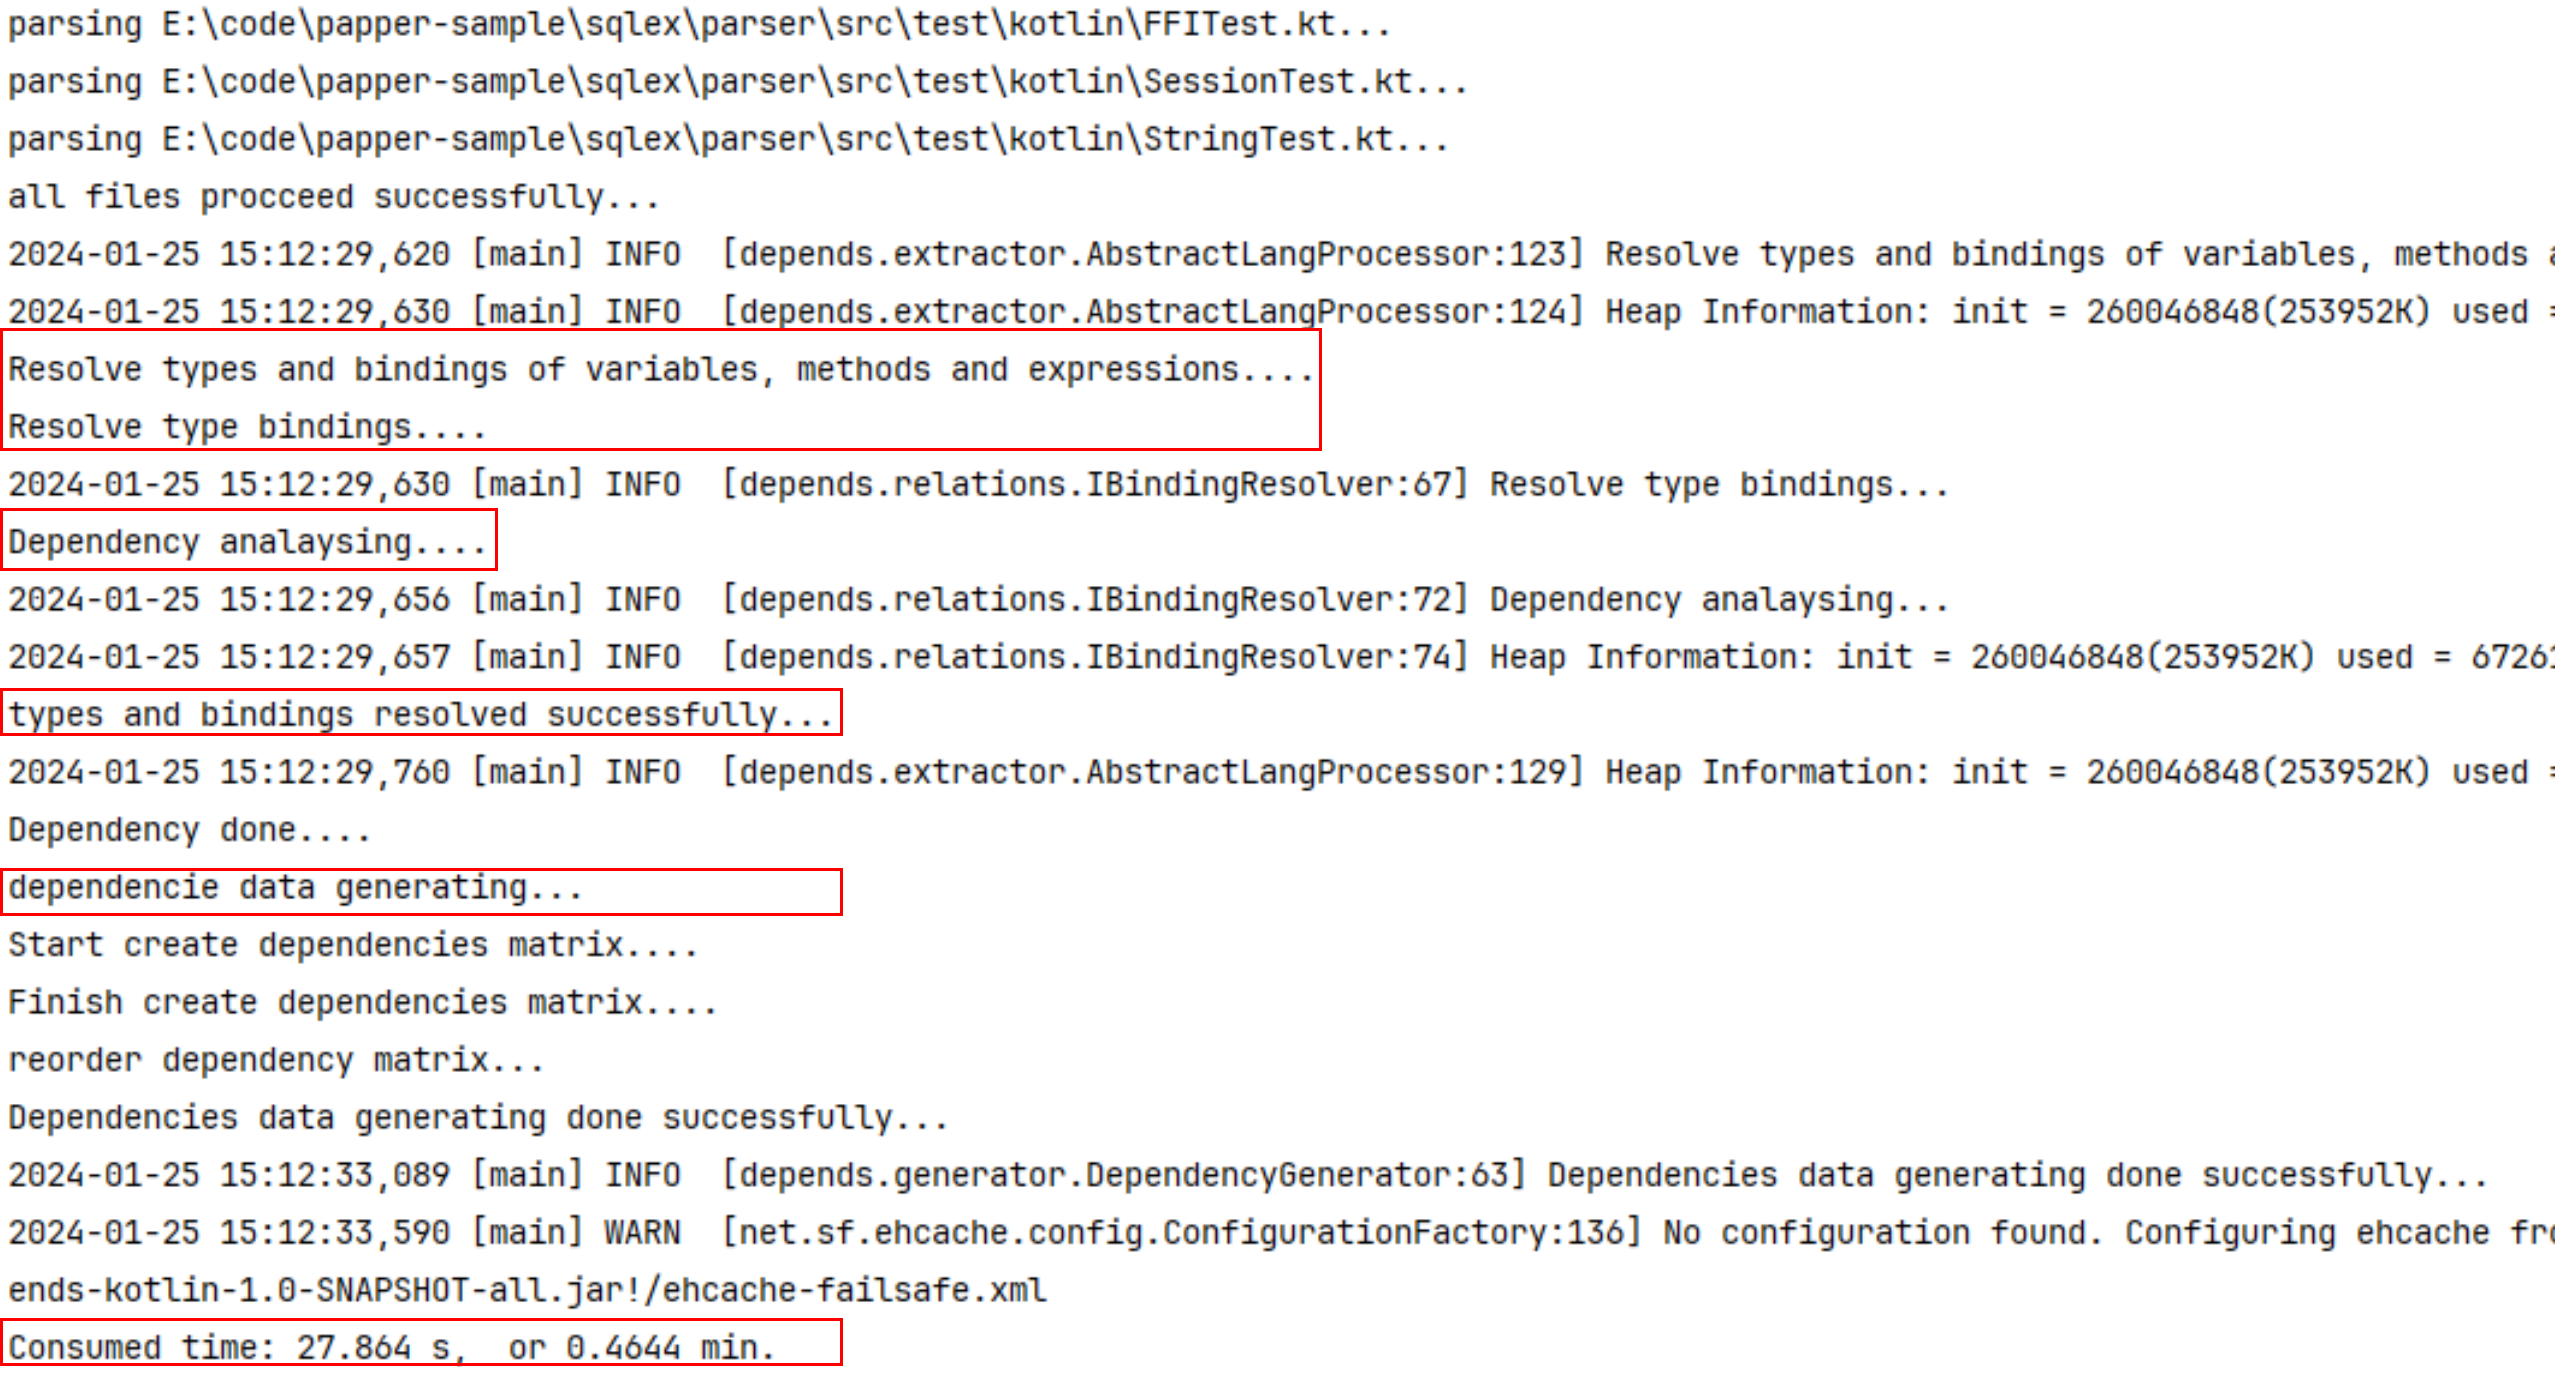}
    \caption{Running screenshot of sqlex.}
    \label{fig:run-log}
\end{figure}

For example, if we need to analyze a Kotlin(-Java) project ``sqlex'', we can execute the command as follows:

\begin{center}
    \lstinline[language=bash]|java -jar depends-kotlin.jar kotlin ./sqlex result -d ./out|\\
\end{center}

\textit{Depends-Kotlin} will analyze the source code in the \texttt{./sqlex} folder and display the running process in the command console as marked in Figure~\ref{fig:run-log}. When the analysis is complete, the console will show the consumed time and the analysis results will be output to the specified folder. In this example, the output (analysis results) of the sqlex project can be found in the \texttt{./out} folder. 

Figure~\ref{fig:result} displays the results of dependency relations at the file level in the output folder. The \texttt{variables} shows an ordered list of file names. The \texttt{cells} shows a random list of dependency relations and each cell displays the dependency relations between two source files. For example, the red rectangle shows entities in \texttt{File 141} \texttt{call} and \texttt{import} entities in \texttt{File 206}.

\begin{figure}[H]
    \centering
    \includegraphics[width=0.9\columnwidth]{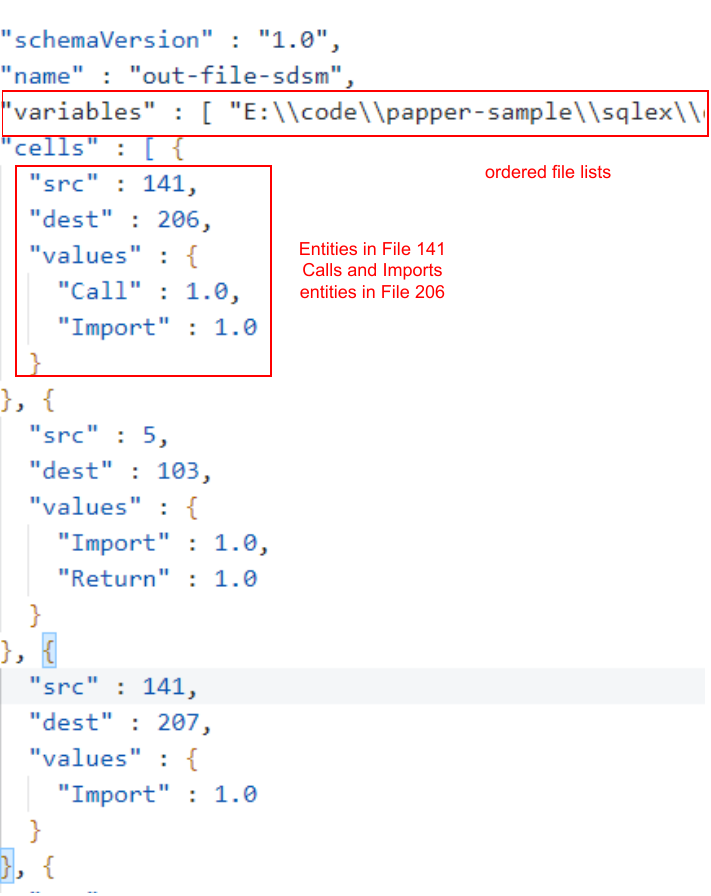}
    \caption{Output screenshot of sqlex's dependency results.}
    \label{fig:result}
\end{figure}

\noindent
